# Supplementary material for: Deviation bound for non-causal machine learning
Source: arXiv:2009.08905 source file (2021-03-19)
Supplement: Supplementary file 1 [file Ising.tex]

In this section, we propose an example of application of our model to a multi dimensional random fields. This example is strongly related to Ising models, that have many applications in physics.

We consider a random field of i.i.d innovations $(\varepsilon_i)$ distributed uniformly on $(0,1)$. We consider a $\kappa$-orthotope $V \subset \mathbb{Z}^{\kappa}$. For $i, j \in V$ note $i \sim j$ if $i$ and $j$ are neighbors in the $\kappa$-dimensional lattice. Let us denote by B $\delta$-neighboorhood on the lattice. We also consider the function $F :\{-1,1\}^B \times (0,1)  \longrightarrow \{-1,1\} $. We consider the following function $F$:

\[F((x_i)_{i \in B}, e) =  2 1_{\varepsilon_i \geq h((X_j)_{j, i \sim j})}-1 \]

where $h((X_j)_{j, i \sim j}) = \frac{\exp(\beta s_i \sum_j X_j)}{\exp(\beta \sum_j X_j) +\exp( - \beta \sum_j X_j) }$

Let $(X_j)$ be a solution of \eqref{masterEquation} f

  and $(\epsilon_i)$ is random field where the marginals are independent and follows an uniform distribution on $(0,1)$. Therefore, $(X_j)_{j, i \sim j}$ follows \eqref{masterEquation}, with $F(X,\varepsilon) = 2 1_{\varepsilon_i \geq h((X_j)_{j, i \sim j})}-1$.

We suppose that the random field is markovian, and verify the Markov property for $\beta > 0$:

\begin{equation}
    \mathbb{P}[X_i =s_i|  X_j, i \sim j ]= \frac{\exp(\beta s_i \sum_j X_j)}{\exp(\beta \sum_j X_j) +\exp( - \beta \sum_j X_j) }
    \label{eq:Markov_field_equation_}
\end{equation}

It is possible to show the following lemma : 
\begin{lem}
For $x = (x_j)_{j, i \sim j})$ and $x^{[s]}$ that differ on a unique index $s \in V$
\[|h(x) - h(x^{[s]})| \leq \lambda(\beta) = \frac{1 }{1 + e^{\beta (n-3)}}\]
where n is the following cardinal $n = \card{\{ j, i \sim j \}}$
\end{lem}

\begin{proof}
Let $y =  \exp(\beta s_i \sum_{j,j \not = s} X_j)$. We have the following relation:
\[|h(x) - h(x^{[s]})| \leq \frac{e^{2 \beta}- e^{-2 \beta}}{e^{2 \beta}+e^{-2 \beta}+ y^2+\frac{1}{y^2}}\]

In every case, at least the half of the values ${X_j,j \not = s}$ is equal to 1, so  $y^2 \geq e^{ \beta(n-1)}$, or at least the half of the values ${X_j,j \not = s}$ is equal to $-1$,so $y^{-2} \geq e^{ \beta(n-1)}$. 

Therefore : 
\[|h(x) - h(x^{[s]})| \leq \frac{1- e^{-4 \beta}}{1+e^{-4 \beta}+e^{ \beta(n-3)}}\]
\end{proof}

Now, we can prove the following lemma:

\begin{proof}
\begin{align*}
    \|F(X, \varepsilon)-F(X^{[s]}, \varepsilon)\|_m 
    & = \esp[2|1_{\varepsilon \geq h(X)} - 1_{\varepsilon \geq h(X^{[s]})}|]^{\frac{1}{m}} \\
    & = 2 \cdot \esp[1_{\varepsilon \in (h(X),h(X^{[s]}))}]^{\frac{1}{m}}\\
    & \leq 2  \\
\end{align*}

\end{proof}
