# Supplementary material for: Deviation bound for non-causal machine learning
Source: arXiv:2009.08905 source file (2021-03-19)
Supplement: Supplementary file 2 [file MCDiarmidExtended.tex]

% preuve du corollaire chinois sur l'extention du MC Diarmid
\begin{proof}
This Lemma is a immediate consequence of the total probability law. \\
We denote $\Bar{A}$ the complement of $A$.
\begin{align*}
    \forall t > 0, & \pr(|f(X_1, \dots, X_n) - \esp\left[ f(X_1, \dots, X_n) | A \right]| \ge t)  \\ 
    & = \pr(|f(X_1, \dots, X_n) - \esp\left[ f(X_1, \dots, X_n) | A \right]| \ge t | A) \pr(A) + \pr(|f(X_1, \dots, X_n) - \esp\left[ f(X_1, \dots, X_n) | A \right]| \ge t | \Bar{A}) \pr(\Bar{A}) \\
    & \leq \pr(|f(X_1, \dots, X_n) - \esp\left[ f(X_1, \dots, X_n) | A \right]| \ge t | A) \pr(A) + 1 - \pr(A).
\end{align*}
On the sub space conditioned by A, f is difference bounded (condition \eqref{equ:strong_difference_bound}), therefore we can apply Mc Diarmid inequality. (see Theorem \ref{ineq:mcDiarmid}).
\begin{equation*}
    \pr(|f(X_1, \dots, X_n) - \esp\left[ f(X_1, \dots, X_n) | A \right]| \ge t | A) \leq \exp \left( \frac{-2t^2}{\sum_{j=1}^N c_j^2} \right).
\end{equation*}
\end{proof}
